# Supplementary material for: Embedding Hindsight Reasoning in Separation Logic
Source: arXiv:2209.13692 source file (2023-04-21)
Supplement: Supplementary file 1 [file lo_proofs_full.tex]

%!TEX root = ../../main.tex

\subsection{Proof Outlines for \texttt{insert} and \texttt{delete}}
\label{sec:lotree:insertion-deletion}
The proof outline for the methods \code{insert} and \code{delete} can be found in \Cref{fig:lotree:impl}.
While the proof requires mostly standard reasoning, it reveals the interference that other threads are subject to.
It is this interference that the hindsight reasoning for method \code{contains} in \Cref{sec:lotree:contains} is relative to.

\lopar{Locating Nodes}
Recall from \Cref{sec:lotree:overview} that \code{insert} and \code{delete} use the helper \code{locate} to find the position $\pprev,\pnext$ to which a given key $\vk$ belongs.
Node $\pprev$ is the result of a tree traversal, \Cref{code:lotree:locate:tree}.
Since we elide the mechanics of the tree overlay, we only know that the resulting pointer is non-$\nullptr$---this little information suffices.
Next, $\pprev$ is locked, \Cref{code:lotree:locate:lock}.
This provides us with the protected resources, $\holds{\pprev}$.
They guarantee that $\succof{\pprev}$, $\markof{\pprev}$, and $\markof{\pnext}$ cannot change due to interference.
Moreover, invoking invariant~\eqref{eq:lotree:inv:succmarkpredflow} just prior to the lock yields $\neg\markvarof{\pprev}\Rightarrow\neg\markvarof{\succvarof{\pprev}}$.
Reading $\succof{\pprev}$, \Cref{code:lotree:locate:next}, binds $\pnext$ to $\succvarof{\pprev}$.
Hence, the validation of position $\pprev,\pnext$ on \Cref{code:lotree:locate:return} results in the interference-free knowledge that both $\pprev$ and $\pnext$ are unmarked, $\pnext$ is the successor of $\pprev$, and that $\vk$ indeed belongs in-between $\pprev$ and $\pnext$, $\vk\in(\keyvarof{\pprev},\keyvarof{\pnext}]$.
This together with the obtained resources forms the predicate $\locateInv(\somenodes,\pprev,\pnext)$, formally defined in \Cref{fig:lotree:impl}, and is the post condition of \code{locate} on \Cref{code:lotree:locate:post}.

Later, we will use the fact that $\locateInv(\somenodes,\pprev,\pnext)$ implies $\vk\in\keysetof{\pnext}$.
To see this, invoke invariant~\eqref{eq:lotree:inv:flow} for the unmarked $\pprev$.
We get $[\keyvarof{\pprev},\infty]\subseteq\insetof{\pprev}$.
The flow $(\keyvarof{\pprev},\infty]$ distributes via $\succof{\pprev}$ to $\pnext$ according to \Cref{sec:lotree:locality}.
Hence, $\vk\in\keysetof{\pnext}=(\keyvarof{\pprev},\keyvarof{\pnext}]$.

\lopar{Insertions}
An Insertion of key $\vk$ first calls \code{locate} to find the position $\pprev,\pnext$ to which $\vk$ belongs.
The position reveals if $\vk$ is already contained because $\vk\in\keysetof{\pnext}$ as inferred above.
If $\keyvarof{\pnext}=\vk$, then $\vk\in\contentsof{\pnext}$ and thus $\vk\in\contentsof{\somenodes}=\abscontent$.
That is, if the conditional in \Cref{code:lotree:insert:check} succeeds, the specification of an unsuccessful insertion is satisfied.
We trade the obligation $\OBLi{\vk}$ for the receipt $\FULi{\false}$.

\input{content/lotree/fig_linkage}

Otherwise, $\vk$ is inserted into the the structure.
To do that, a new node $\pnode$ containing $\vk$ is allocated in \Cref{code:lotree:insert:malloc}.
The $\predsel$ resp. $\succsel$ fields are set to $\pprev$ resp. $\pnext$.
It remains to link $\pnode$ into the logical ordering, as depicted in \Cref{fig:illustration-insertion}.
First, \Cref{code:lotree:insert:linksucc} redirects $\succof{\pprev}$ to $\pnode$.
This is the linearization point: $\pnode$ receives the flow $(\keyvarof{\pprev},\infty]$ from $\pprev$ so that we have $\set{\vk}=\contentsof{\pnode}\subseteq\keysetof{\pnode}$.
Hence, the update turns $\abscontent$ into $\abscontent\cup\set{\vk}$ so that $\OBLi{\vk}$ can be traded for $\FULi{\true}$.
Next, \Cref{code:lotree:insert:linkpred} redirects $\predof{\pnext}$ to $\pnode$.
The command has no effect on the logical contents $\abscontent$ which is why we need no $\OBLi{\vk}$ to proceed.
It is readily checked that the update maintains the node-local invariants of the nodes $\pprev,\pnode,\pnext$.

Our proof outline does not consider the methods for inserting the new node $\pnode$ into the tree overlay.
We simply assume that \code{prepareTreeInsertion} in \Cref{code:lotree:insert:preparetree} produces an interference-free predicate $\hiddenIns{\pprev,\pnext}$ that is maintained by the updates of the logical ordering in \Cref{code:lotree:insert:linksucc,code:lotree:insert:linkpred} and consumed by the later \code{performTreeInsertion} in \Cref{code:lotree:insertIntoTree}.

\lopar{Deletions}
Deletions are similar to insertions.
They first \code{locate} the position $\pprev,\pcurr$ to which $\vk$ belongs.
If $\vk\in\contentsof{\pcurr}$, then $\vk\in\abscontent$.
In this case the conditional on \Cref{code:lotree:delete:check} is successful and we can trade $\OBLd{\vk}$ for $\FULd{\false}$.
Otherwise, $\pcurr$ is locked, \Cref{code:lotree:delete:lock}.
This gives the necessary resources to modify $\pcurr$'s $\marksel$, $\predsel$, and $\succsel$ fields.
\Cref{code:lotree:delete:mark} first marks $\pcurr$.
This is the moment the logical deletion takes place: it changes $\contentsof{\pcurr}=\set{\vk}$ to $\contentsof{\pcurr}=\emptyset$ and thus changes $\abscontent$ to $\abscontent\setminus{\vk}$.
Hence, we can turn $\OBLd{\vk}$ into $\FULd{\true}$.
Next, $\pcurr$ is physically unlinked from the logical ordering, as depicted in \Cref{fig:illustration-deletion}.
The unlinking reverses the linking performed by \code{insert}.
That $\pcurr$ is guaranteed to have an empty inset after the unlinking is due to invariant~\eqref{eq:lotree:inv:flow}.
With this, it is easy to check that the updates do not modify the logical contents and maintain the node-local invariants of the nodes $\pprev,\pnode,\pnext$.

As for \code{insert}, we do not consider the deletion of $\pcurr$ from the tree overlay.
We simply assume that \code{prepareTreeDeletion} in \Cref{code:lotree:delete:preparetree} produces an interference-free predicate $\hiddenDel{\pcurr}$ that is maintained by the updates of the logical ordering in \Cref{code:lotree:delete:mark,code:lotree:delete:unlinkpred,code:lotree:delete:unlinksucc} and consumed by the later \code{performTreeDeletion} in \Cref{code:lotree:removeFromTree}.

% =================================================================================================
% =================================================================================================
% =================================================================================================
% =================================================================================================
% =================================================================================================
\subsection{Proof Outline and Temporal Interpolation for \texttt{contains}}
\label{sec:lotree:contains}

The proof outline and hindsight arguments for method \code{contains($\vk$)} appear in \Cref{fig:lotree:proof-contains} (the figure repeats the implementation of \code{contains} from \Cref{fig:lotree:impl}).
The proof uses implicitly existentially quantified symbolic variables $\anodeval,\anodevalp,\avalval$ to share knowledge between now and past predicates.
We cannot use program variables for this purpose because their values change during computation, meaning they may be valuated differently in now and past predicates.
To further avoid confusion between now and past states, we write $\old{e}$ to replace in expression $e$ all symbolic variables like $\markof{\anodeval}$ with $\old{\markof{\anodeval}}$.
We think of $\old{e}$ as the \emph{old} version and use it under past operators.
For example, in $\nowof{\inv(\abscontent,\set{\anodeval})}\mstar\pastof{\old{\inv(\abscontentp,\set{\anodeval})}}$ we would use $\insetof{\anodeval}$ resp. $\old{\insetof{\anodeval}}$ to clearly refer to the inset of $\anodeval$ in the current resp. past state.
The proof has these five stages:
\begin{asparaenum}[(1)]
	\item\label{lotree:stage-treetraverse}
		The tree traversal, \Cref{code:lotree:contains:treetraversal}, finds a starting node $\pcurr$ for traversing the logical ordering.
		The only guarantee for the resulting $\pcurr$ is that it is non-$\nullptr$, \Cref{code:lotree:contains:treetraversal-post}.
	\item\label{lotree:stage-fix}
		The logical ordering is traversed by following $\predsel$ fields until an unmarked node is reached, \Cref{code:lotree:contains:fix}.
		The resulting node $\pcurr$ is non-$\nullptr$ by invariant~\eqref{eq:lotree:inv:contents-closed}.
		That it is unmarked means that it has flow by invariant~\eqref{eq:lotree:inv:flow}, $\insetof{\pcurr}\neq\emptyset$.
		This fact is not interference-free because $\pcurr$ is not locked.
		To preserve this, we turn it into a past predicate, \Cref{code:lotree:contains:go-pred-pre}.
	\item\label{lotree:stage-gopred}
		The traversal continues to follow $\predsel$ pointers as long as $\vk$ is less than the key in the traversed node, \Cref{code:lotree:contains:go-pred}.
		Using temporal interpolation (see below), we show that following $\predsel$ pointers maintains the past flow information so that the reached node $\pcurr$ is known to have had flow at some point.
		Together with invariant~\eqref{eq:lotree:inv:flow} and $\vk \geq \keyof{\pcurr}$, we obtain $\vk\in\insetof{\pcurr}$, \Cref{code:lotree:contains:go-succ-pre}.
		So we are \emph{on track} to find $\vk$.
	\item\label{lotree:stage-gosucc}
		The traversal follows $\succsel$ pointers as long as $\vk$ is greater than the key in the traversed node, \Cref{code:lotree:contains:go-succ}.
		Using temporal interpolation (see below), we conclude that also the reached node $\pcurr$ had $\vk$ in its inset at some point.
		Note that this together with $\vk\leq\keyof{\pcurr}$ from \Cref{code:lotree:contains:go-succ-post} means $\vk\in\keysetof{\pcurr}$ in some past state.
		So $\vk$ was in the structure at this past state iff it was in $\contentsof{\pcurr}$.
	\item\label{lotree:stage-check}
		Using temporal interpolation (see below), we derive from the past contents and the current $\keysel$ and $\marksel$ fields of $\pcurr$ whether or not $\vk$ has been in the logical contents of the structure, \Cref{code:lotree:contains:validate}.
		This past state is, in fact, the linearization point.
		We retrospectively linearize, \Cref{code:lotree:contains:final}, before returning.
\end{asparaenum}

We turn to the details of the temporal interpolation that goes into obtaining the proof outline for the last three stages as described above.

%!TEX root = ../../main.tex

\begin{wrapfigure}{r}{.465\textwidth}
	\vspace{-2mm}

	\begin{lstlisting}[language=compactSPL,aboveskip=-4.25mm,numbers=none]
$\makeTeal{\begin{aligned}[t]&
	\succInv(\abscontent,\abscontentp\!\!,\somenodes,\somenodesp,\anode,\anodeval) \,\defeq\,
		\inv(\abscontent,\somenodes\cup\anodeval) \MYMSTAR \anode=\anodeval
		\mkNL \MYMAND
		\pastOF{ \old{\inv(\abscontentp\!\!,\somenodesp\cup\anodeval)} \MYMSTAR \vk\in\old{\insetof{\anodeval}} }
\end{aligned}}$
\end{lstlisting}
			\begin{lstlisting}[language=compactSPL,belowskip=-2mm]
$\ANNOT{\exists \abscontent,\somenodes.~ \OBLc{\vk} \MYMSTAR \inv(\somenodes) \MYMSTAR -\infty < \vk < \infty }$
method contains($\vk$: Int): Bool {
	val $\pcurr$ = traverse($\vk$)   $\label{code:lotree:contains:treetraversal}$
	$\ANNOT{ \OBLc{\vk} \MYMSTAR \travInvOf{\pcurr} }$   $\label{code:lotree:contains:treetraversal-post}$
	while ($\vk$ < $\pcurr$.key)@\:@{@\:@val $\pprev$@\;@=@\;@$\pcurr$.pred;@\:@$\pcurr$@\;@:=@\;@$\pprev$@\:@}   $\label{code:lotree:contains:go-pred}$
	$\ANNOT{ \OBLc{\vk} \MYMSTAR \travInvOf{\pcurr} \MYMSTAR \keyvarof{\anodeval}\leq\vk }$ $\label{code:lotree:contains:go-pred-post}$
	while ($\pcurr$.mark)@\:@{@\:@val $\pprev$@\;@=@\;@$\pcurr$.pred;@\:@$\pcurr$@\;@:=@\;@$\pprev$@\:@}   $\label{code:lotree:contains:fix}$
	$\ANNOTML{ &\OBLc{\vk} \MYMSTAR \travInvOf{\pcurr} \\&\MYMSTAR \keyvarof{\anodeval}\leq\vk \MYMSTAR \neg\markvarof{\anodeval} }$   $\label{code:lotree:contains:fix-post}$
	$\ANNOT{ \OBLc{\vk} \MYMSTAR \succInvOf{\pcurr} }$   $\label{code:lotree:contains:go-succ-pre}$
	while ($\pcurr$.key < $\vk$)@\:@{@\:@val $\pnext$@\;@=@\;@$\pcurr$.succ;@\:@$\pcurr$@\;@:=@\;@$\pnext$@\:@}   $\label{code:lotree:contains:go-succ}$
	$\ANNOT{ \OBLc{\vk} \MYMSTAR \succInvOf{\pcurr} \MYMSTAR \vk\leq\keyvarof{\anodeval} }$   $\label{code:lotree:contains:go-succ-post}$
	val $\vres$ = $\pcurr$.key == $\vk$   $\label{code:lotree:contains:validate}$
	$\ANNOTML{
		& \OBLc{\vk} \MYMSTAR \inv(\abscontent,\somenodes) \MYMSTAR \vres=\avalval 
		\\& \MYMSTAR 
		\pastOf{
			\old{\inv(\abscontentp\!\!,\somenodesp)} \MYMSTAR
			% \avalval \Leftrightarrow \vk\prall{\in}\old{\contentsof{\somenodesp}}=\abscontentp
			\avalval \Leftrightarrow \vk\prall{\in}\abscontentp
		}
	}$   $\label{code:lotree:contains:validate-annot}$
	$\ANNOT{ \FULc{\vres} \MYMSTAR \inv(\abscontent,\somenodes) }$   $\label{code:lotree:contains:final}$
	return $\vres$   $\label{code:lotree:contains:return}$
}
$\ANNOT{\vres.~ \exists \abscontent,\somenodesp.~ \FULc{\vres} \MYMSTAR \inv(\abscontent,\somenodes) }$
\end{lstlisting}
	\caption{
		Proof outline for method \code{contains}.
		The temporal interpolation required for the loop on \Cref{code:lotree:contains:go-succ} is detailed in \Cref{fig:lotree:hindsight-succ}.
		\label{fig:lotree:proof-contains}
	}
\end{wrapfigure}

%%% Local Variables:
%%% mode: latex
%%% TeX-master: "../../main"
%%% End:

% -----------------------------------------------------------------------------
% -----------------------------------------------------------------------------
\lopar{Temporal Interpolation in Stage~\eqref{lotree:stage-gopred}}
The proof outline for the loop from \Cref{code:lotree:contains:go-pred} is given in \Cref{fig:lotree:hindsight-pred}.
The temporal interpolation needed here is this: that $\pcurr$ had flow in the past and that its $\predsel$ field currently points to $\pprev$ means that both facts were true simultaneously at some point.
Intuitively, this is the case because $\pcurr$ has flow whenever $\predof{\pcurr}$ is changed.
Technically, we show the hypothesis $\weakhypof{\apred}{\apredp}{\apred\cap\apredp}$ on \Cref{code:lotree:hindsight-pred:inter-hyp} with
\[
	\apred ~\defeq~ \inv(\abscontentp,\somenodesp\cup\anodeval) \MSTAR \insetof{\anodeval}\neq\emptyset
	\qquad\text{and}\qquad
	\apredp ~\defeq~ \inv(\abscontent,\somenodes\cup\anodeval) \MSTAR \predvarof{\anodeval}=\anodevalp
	\ .
\]
The symbolic variables $\anodeval$ resp. $\anodevalp$ are bound to $\pcurr$ resp. $\pprev$ by the outer proof context; we use $\anodeval$/$\anodevalp$ instead of $\pcurr$/$\pprev$ as they are logically pure and thus do not change their valuation.
To prove the hypothesis, we establish $\thePredicates,\theInterference\semcalc\hoareof{\acpred}{\stmtof{\theInterference}}{\nowof{\apredp}\rightarrow\weakpastOf{\apred\cap\apredp}}$ and $\isInterferenceFreeOf[\theInterference]{\thePredicates}$ for some set $\thePredicates$ of predicates with $\nowof{\apred}\subseteq\acpred\in\thePredicates$~(cf. \Cref{Section:TemporalInterpolation}).
We cannot simply chose $\acpred=\nowof{\apred}$ because $\apred$ is not interference-free.
Instead, we choose $\acpred\defeq\nowof{\apredp}\rightarrow\weakpastOf{\apred\cap\apredp}$.
It is easy to see that $\acpred$ is indeed weaker than $\nowof{\apred}$, $\nowof{\apred}\subseteq\acpred$.
While this choice may be surprising, it is in line with the spirit of temporal interpolation: its goal is to make visible the intermediary states that the interference produced but the isolated thread did not observe.
Note that $\acpred$ is the invariant that the hypothesis proof strategy from \Cref{Lemma:ProofStrategy} asks for.

Next, we show that $\acpred$ is interference-free, i.e., $\csemOf{(\acpredpp,\acom)}(\acpred)\subseteq\acpred$ for all interferences $(\acpredpp,\acom)\in\theInterference$ of the LO-tree.
For an interference $(\acpredpp,\acom)$ to invalidate $\acpred$ it must change the truth of $\apredp$ in the current state.
If the truth of $\apredp$ is changed to $\false$, then $\acpred$ is vacuously true.
Otherwise, the interference changes $\predvarof{\anodeval}$ to $\anodevalp$.
This means $\acom$ stems from \Cref{code:lotree:fix-insert-pred} in \code{insert} or \Cref{code:lotree:delete:unlinkpred} in \code{delete}.
In both cases we know from the proof discussed in \Cref{sec:lotree:insertion-deletion} (\Cref{fig:illustration-insertion,fig:illustration-deletion}) that $\anodeval$ has flow after the interfering update.
Concretely, this means $\csemOf{(\acpredpp,\acom)}(\acpred)\subseteq\nowof{\apred}$.
Because we already established $\nowof{\apred}\subseteq\acpred$, we obtain the interference-freedom of $\acpred$, as required.

It remains to show that $\acpred$ is invariant under the self-interferences $\stmtof{\theInterference}$.
To see this, observe that $\acpred$ concerns only the global state, not the local state.
Hence, the self-interferences invalidate $\acpred$ iff the interferences of other threads do so.
Since the latter is not the case, nothing needs to be shown.

With the hypothesis proved, we obtain $\pastOf{\apred\cap\apredp}$ from Rule~\ruleref{temporal-interpolation}.
The rule is applied to a command which we make explicit in the form of the $\cskip$ on \Cref{code:lotree:hindsight-pred:skip}.
One can avoid this skip by applying the rule together with the previous command.
Finally, the desired assertion on \Cref{code:lotree:hindsight-pred:inter-post}, namely $\pastOf{\inv(\abscontentp,\somenodesp\cup\anodevalp) \mstar \insetof{\anodevalp}\neq\emptyset}$, follows from applying the invariants \eqref{eq:lotree:inv:contents-closed} and \eqref{eq:lotree:inv:succmarkpredflow}.

% -----------------------------------------------------------------------------
% -----------------------------------------------------------------------------
\lopar{Temporal Interpolation in Stage~\eqref{lotree:stage-gosucc}}
The proof outline for the loop from \Cref{code:lotree:contains:go-succ} is given in \Cref{fig:lotree:hindsight-succ}.
We elaborate only briefly as the line of argument is similar to the one from Stage~\eqref{lotree:stage-gopred}.
The interpolation goal is to show that $\vk\in\insetof{\pcurr}$ has been preserved at least up to the moment the current value of $\succof{\pcurr}$ was installed.
The hypothesis for this is $\weakhypof{\apred}{\apredp}{\apred\cap\apredp}$ on \Cref{code:lotree:hindsight-succ:inter-hyp} with
\[
	\apred ~\defeq~ \inv(\abscontentp,\somenodesp\cup\anodeval) \MSTAR \vk\in\insetof{\anodeval}
	\qquad\text{and}\qquad
	\apredp ~\defeq~ \inv(\abscontent,\somenodes\cup\anodeval) \MSTAR \succvarof{\anodeval}=\anodevalp \MSTAR \keyvarof{\anodeval} < \vk
	\ .
\]
We invoke \Cref{Lemma:ProofStrategy} again with the canonical invariant $\acpred\defeq\nowof{\apredp}\rightarrow\weakpastOf{\apred\cap\apredp}$.
It is readily checked that $\nowof{\apred}\subseteq\acpred$ holds.
Interference freedom holds for $\acpred$ if it is preserved by interferences that change $\succvarof{\anodeval}$; $\keysel$ fields never change which is why the truth of $\keyvarof{\anodeval} < \vk$ cannot change (for simplicity, we treat $\vk$ as a symbolic variable).
Such interferences are due to \Cref{code:lotree:insert:linksucc} in \code{insert} and \Cref{code:lotree:delete:unlinksucc} in \code{delete}.
From the proof outline in \Cref{sec:lotree:insertion-deletion} we know that in both cases we have $\vk\in\insetof{\anodeval}$ because updating $\succsel$ does not change the node's flow (cf. \Cref{fig:illustration-insertion,fig:illustration-deletion}).
This means the interference results in a state satisfying $\nowof{\apred}\subseteq\acpred$, as required.
Again, there is nothing to show for self-interferences because $\acpred$ is a purely global property.
Hence, we obtain the assertion on \Cref{code:lotree:hindsight-succ:inter-post}.

% -----------------------------------------------------------------------------
% -----------------------------------------------------------------------------
\lopar{Temporal Interpolation in Stage~\eqref{lotree:stage-check}}
We proceed in two steps.
First, we prove the hypothesis $\weakhypof{\apred}{\apredp}{\apred\cap\apredp}$ for arbitrary $\apred$ and $\apredp\defeq\keyvarof{\anodeval}=\avalval$.
As before, we use \Cref{Lemma:ProofStrategy} with invariant $\acpred\defeq\nowof{\apredp}\rightarrow\weakpastOf{\apred\cap\apredp}$.
Since $\keyvarof{\anodeval}$ is immutable (it never changes), we immediately obtain that $\acpred$ is stable under self-interferences and interferences from other threads.
This justifies to move knowledge about the $\keysel$ freely between now and past predicates.
In fact, we use this reasoning to derive the transition from \Cref{code:lotree:contains:go-pred-post} to \Cref{code:lotree:contains:go-succ-pre}.

Towards \Cref{code:lotree:contains:validate-annot}, consider the case where $\keyvarof{\anodeval}\neq\vk$ first.
Together with $\vk\leq\keyvarof{\anodeval}$ from \Cref{code:lotree:contains:go-succ-post}, we have $\vk<\keyvarof{\anodeval}$.
As before, we move this into the past predicate from \Cref{code:lotree:contains:go-succ-post}.
The result is $\pastOf{\old{\inv(\abscontentp,\somenodesp)}\mstar\vk\in\old{\insetof{\anodeval}}\mstar\vk\neq\old{\keyvarof{\anodeval}}}$.
By definition, $\vk\in\old{\keysetof{\anodeval}}$ and $\vk\notin\old{\contentsof{\anodeval}}$ hold in the past state.
Hence, $\pastOf{\old{\inv(\abscontentp,\somenodesp)}\mstar\vk\notin\old{\contentsof{\somenodesp}}}$ follows from the invariant.

Next, consider $\keyvarof{\anodeval}=\vk$ and $\markvarof{\anodeval}=\true$.
We obtain $\pastOf{\old{\inv(\abscontentp,\somenodesp)}\mstar\vk=\old{\keyvarof{\anodeval}}}$ from interpolation.
Another interpolation wrt. $\markvarof{\anodeval}=\true$ yields $\pastOf{\old{\inv(\abscontentp,\somenodesp)}\mstar\vk=\old{\keyvarof{\anodeval}}\mstar\old{\markvarof{\anodeval}}}$.
The corresponding hypothesis follows as easily as in the case of $\keysel$ fields since $\markvarof{\anodeval}=\true$ is immutable ($\marksel$ fields may change, however, once set to $\true$ they remain $\true$).
Overall, we derive that $\vk$ is not contained in the structure in the past: $\pastOf{\old{\inv(\abscontentp,\somenodesp)}\mstar\vk\notin\contentsof{\somenodesp}}$.

The remaining case is $\keyvarof{\anodeval}=\vk$ and $\markvarof{\anodeval}=\false$.
This case does not require temporal interpolation reasoning.
It suffices to invoke invariant \eqref{eq:lotree:inv:flow}.
We obtain $\nowOf{\inv(\abscontent,\somenodes\cup\anodeval)\mstar\keyvarof{\anodeval}\in\contentsof{\somenodes}}$.

Rewriting the three cases from above yields the assertion from \Cref{code:lotree:contains:validate-annot}.
Moreover, it allows the method to retrospectively linearize as the past predicate witnesses a past state of the structure where $\vk$ was resp. was not in the structure as reflected by the return value.
This concludes the linearizability proof of method \code{contains}.
